# Supplementary material for: Numerical Study of Eigenvector Deflation to Accelerate the WaveHoltz Method
Source: arXiv:2606.31842 source file (2026-06-30)
Supplement: Supplementary file 1 [file appendix.tex]

%!TEX root = ../deflation.tex
%%%%%%%%%%%%%%%%%%%%%%%%%%%%%%%%%%%%%%%%%%%%%%
\section{$A$-orthogonality with exact eigenvector deflation\label{sec:A-orthogonality}}
%%%%%%%%%%%%%%%%%%%%%%%%%%%%%%%%
Here, we show that, when $W$ comprises exact eigenvectors of $\whiA_h$, there is no need to  impose $A$-orthogonality in DCG, as $A$-orthogonality is auntomatically guaranteed.

Expand $\rb_0$ as a linear combintation of eigenvectors $\rb_0=\sum_{j=1}^N r_j\wb_j$.
Since $W^T\rb_0=0$ we have $r_j=0$ with $j=1,\dots,K$. As a result 
\begin{equation*}
W^TA \rb_0 = \sum_{j={K+1}}^N W^T \lambda_j r_j\wb_j =0.
\end{equation*}
This guarantees ${\bm \mu_0}=0$ and $W^T \pb_0=0$. With mathematical induction one can show that ${\bm \mu_k}=0$ and $W^T\pb_{k}=W^T\rb_{k}=0$ for any $k$.

%%%%%%%%%%%%%%%%%%%%%%%%%%%%%%%
% \bibliographystyle{plain}
% \bibliography{ref}

%%%%%%%%%%%%%%%%%%%%%%%%%%%%%%%%%%%%%%%%%%%%%%
\clearpage
%%%%%%%%%%%%%%%%%
%\begin{comment}
%%%%%%%%%%%%%%%%%
\subsubsection{Accuracy needed for $(W^TAW)^{-1}$}
We need to apply $(W^TAW)^{-1}$ when we construct $\xb_0$ or impose $A$-orthogonality with respect to the deflation space to the search directions $\pb_k$. Here we will discuss how we implement $(W^TAW)^{-1}$ operation in practice.

When $W$ is formed eigenvectors of $A$, one can prove that $W^TAW$ is a diagonal matrix whose diagonal elements are the corresponding eigenvalues, and it is simple and computationally cheap to invert such a $W^TAW$.
When the size of $W^TAW$, $K$ is much smaller than $N$, we can directly factorize it to compute $W^TAW)^{-1}$. 
For a larger $W^TAW$, we can use a Krylov subspace iterative solver to invert it. The required accuracy for such solvers is numerically investigated in \cite{nabben2006comparison}, analyzed and further relaxed in \cite{kahl2017deflated}. The analysis in \cite{kahl2017deflated} suggests that given the sopping criterion for the DCG algorithm
$||\rb_k||\leq \varepsilon \bbb$, 
the required accuracy for the inner loop solving the linear system determined by $W^TAW$ is
\begin{equation}
    ||\rb_k^{\textrm{inner}}||\leq c\frac{\varepsilon}{||\rb_k||}||\bbb^{\textrm{inner}}|||,\quad 0\leq c<1.
\end{equation}
As the iteration continues, the residual in the DCG algorithm $||\rb_k||$ becomes smaller and the required accuracy for the inner loop solving $W^TAW$ can be adaptively enlarged.

\subsection{Eigenvalues for different geometries} (\textcolor{blue}: we should remove this Section)
The geometry of $\Omega$ affects the distribution and values of the eigenvalues of the $S$ operator. Here, we present the eigenvalues for a few different geometries.

\subsubsection{The Unit Square in $d$-dimensions}
The eigenvalues and eigenvectors of the three point discretization $[-1, 2, -1]$ of the Laplacian on $[0,1]$ with a grid size $h=1/(n+1)$ with Dirichlet boundary conditions are
\begin{eqnarray}
    \lambda_k &= 2 \left(1-\cos \left(\frac{k \pi}{n+1}\right) \right),\ \ k = 1\ldots,n \\
    w_k[i] &= \sqrt{\frac{2}{n+1}} \sin\left(i\frac{k\pi}{n+1}\right),\ \  i = 1\ldots,n,\, k = 1\ldots,n. 
\end{eqnarray}

\begin{figure}[htb]
\begin{center}
\includegraphics[width=0.46\textwidth,trim={0.0cm 0.0cm 0.0cm 0.0cm},clip]{figures/beta_eig_contour_2d}
\includegraphics[width=0.5\textwidth]{figures/beta_eig_contour_3d}
\caption{Number of eigenvectors needed to reach $\beta_\omega(\lambda)<\beta$. Left: 2D. Right: 3D. \label{fig:beta_omega_contour}}
\end{center}
\end{figure}

\begin{figure}[htb]
\begin{center}
\includegraphics[width=0.5\textwidth]{figures/omega_ap_contour_2d}
\caption{Number of eigenvectors needed to reach $\beta_\omega(\lambda)<0.95$. \label{fig:beta_omega_contour}}
\end{center}
\end{figure}

\subsection{Multilevel DCG}
Constructing eigenvector deflation matrix may be costly especially when a refined grid is used. To mitigate this computational cost, we can design a multilevel DCG method which first converts $\whiA\xb=\bbb$ to a problem on a coarse grid  and then performs the eigenvector deflation on the coarse grid where the eigenvectors can be more efficiently computed.  

Multilevel DCG method can be designed following \cite{kruzik2017wavelet,kruvzik2018implementace}. Given a hierarchy of deflation matrix $W_l\in\mathbb{R}^{K_{l-1}\times K_l}$ with $l=1,\dots,L$ and $K_0=N$. Then the deflation matrix and the corresponding Galerkin matrix for the multilevel method are
\begin{equation*}
W = W_1W_2\dots W_L \quad\text{and}\quad W_L^T\dots W_2^T W_1^TAW_1W_2\dots W_L.
\end{equation*}
When solving $A\xb=\bbb$ we apply the DCG method with deflation matrix $W_1$, namely DCG($A,\bbb,W_1$). Inside DCG($A,\bbb,W_1$) we invert $W_1^TAW_1$ with a second DCG solver DCG($W_1^TAW_1,\cdot,W_2)$. We nest the DCG solve until we reach the last level $L$ and invert $W_L^TAW_L$ with a direct or Krylov solver.

Particularly we will apply the following prolongation based deflation (PED) when inverting the WaveHoltz linear system. For $l=1,\dots,L-1$, we choose $W_l$ as a prolongation from a coarse grid with $h_l=2^lh$ to a fine grid with $h_{l-1}=2^{l-1}h$ and choose $W_L$ as eigenvectors of the Galerkin matrix $W_{L-1}^T\dots W_1^T A W_1\dots W_{L-1}^T$ on the most coarse level. The eigenvectors will be only computed on the most coarse grid and there is no need to impose the $A$-orthogonality in the DCG solve for $W_{L-1}^T\dots W_1^T A W_1\dots W_{L-1}^T$.

\begin{rem}
The multilevel DCG described above may be combined with the aforementioned idea of approximating eigenvectors based on information provided by successive solves of multiple right hand side \cite{saad2000deflated,stathopoulos2010computing}, and this combination is left for future investigation.    
\end{rem}

\subsection{Prolongation based eigenvector deflation for the WaveHoltz matrix $\whiA_h$}
Here we define a prolongation eigenvector deflation based a the linear prolongation, and we will find the eigenvectors for the most coarse Galerkin matrix $W_L^TW_{L-1}^T\dots W_1^T\whiA_h W_1W_2\dots W_L$. 

For simplicity we consider $1D$ Helmholtz problem $c(x)\equiv1$.
We first introduce the following grid. Assume $N$ be an even integer. Let $\Omega_h$ be a fine grid: $0=x_0\leq x_1 = h\leq \ldots\leq x_N=1$. Let $\Omega_{2h}$ be the coarse grid:
$0=x^c_0\leq x^c_1 = 2h\leq \ldots\leq x^c_{N/2}=1$. 
The fine grid  $\Omega_h$ and coarse grid $\Omega_{2h}$ with $N=8$ are illustrated in Fig. \ref{fig:fine-coarse-grid}. 
 Let $L_h$ denote the matrix corresponding to the $[-1,2,-1]$ central difference discretization  of $\Delta$ with the mesh size $h=\frac{1}{N}$.

We define the linear prolongation operator $I_{2h}^h$ which maps a grid function $\vb^{2h}$ on the coarse grid $\Omega_{2h}$ to a grid function  on the fine grid $\Omega_h$:
\begin{subequations}
    \begin{align}
    &I_{2h}^h\vb^{2h}_{2j} = \vb^{2h}_j,\;0\leq j\leq\frac{N}{2},\\
    &I_{2h}^h\vb^{2h}_{2j+1} =\half\left( \vb^{2h}_{j}+\vb^{2h}_{j+1}\right),\;0\leq j\leq\frac{N}{2}-1.
    \end{align}
\end{subequations}
The full weighting restriction operator mapping a grid function $\vb^h$ on $\Omega_h$ to a grid function $\Omega_{2h}$ is defined as:
\begin{equation}
(I_{h}^{2h}\vb^h)_{j}=\frac{1}{4}(\vb^h_{j-1}+2\vb^h_{j}+\vb^h_{j+1}), \; 1\leq j\leq \frac{N}{2}-1.
\end{equation}
The full weighting restriction $I_{h}^{2h}$ and the linear prolongation $I_{2h}^h$ satisfy the variational relation: 
\begin{equation}
    I_{h}^{2h} = \frac{1}{2} (I_{2h}^h)^T.\label{eq:variational_property}
\end{equation}
Since in the DCG algorithm $W_l^T$ only appears in $(W^TAW)^{-1}W^T$ terms one can actually replace $W_l^T$ with the restriction operator $I_{2^{l-1}h}^{2^lh}$ when implementing the algorithm.

In the $L$ level prolongation based eigenvector deflation we choose deflation matrices as
\begin{equation}
W_l = \begin{cases}
       I_{2^lh}^{2^{l-1}h}, \quad &1\leq l\leq L-1,\\ 
       \textrm{first $K$ eigenvectors of }W_{L-1}^T\dots W_1^T A W_1\dots W_{L-1}, \quad &l= L. 
       \end{cases}
\end{equation}
With $\whiA_h$ equal to the WaveHoltz operator $I-S_h$, we will show that the eigenvectors for $W_{L-1}^T\dots W_1^T \whiA_h W_1\dots W_{L-1}$ are the eigenvectors of the discrete Laplacian operator on the most coarse grid, $L_{2^Lh}$. 

\subsubsection{Eigenvectors of $W_{L-1}^T\dots W_1^T \whiA_h W_1\dots W_{L-1}$}
We start with proving eigenvectors of $W_1^T\whiA_h W_1$ are the eigenvectors of the discrete Laplacian operator $L_{2h}$. With the variational property \eqref{eq:variational_property}, it is enough to find eigenvectors for $I^{2h}_{h}\whiA I_{2h}^h$. 

The proof is based on the properties of the full weighting restriction and the linear prolongation \cite{briggs2000multigrid}. Let $\wb^h_k$ be an eigenvector of the discrete Laplacian operator $L_{h}$.
\begin{lem}\label{lem:restriction_and_prolong_effect}
Let $k'=N-k$. For $1\leq k < \frac{N}{2}$, following relations are satisfied:
\begin{subequations}
\label{eq:restri_prolong_equality}
\begin{align}
    I_{2h}^{h} \wb^{2h}_k &= c_k^{2h}\wb_k^h-s_k^{2h}\wb_{k'}^h,\label{eq:full_weight} \\
    I_{h}^{2h}\wb^h_k &= c_k^{2h}\wb_k^{2h},\label{eq:prolong_k}\\
    I_{h}^{2h}\wb^h_{k'} &= - s_k^{2h}\wb_k^{2h},\label{eq:prolong_kp}
\end{align}
\end{subequations}
where $c_k^{2h}=\cos^2(\frac{k\pi}{2N})$ and $s_k^{2h}=\sin^2(\frac{k\pi}{2N})$.
\end{lem}

\begin{thm}
Let $1\leq k< \frac{N}{2}$  and $L_{2h}\wb^{2h}_{k}=\sigma_k^2\wb^{2h}_{k}$. Then $\wb^{2h}_k$ is also an eigenvector of $I_{h}^{2h} \whiA_h I_{2h}^h$ with $\whiA_h$ being the WaveHoltz operator on $\Omega_h$ and 
\begin{equation}
I_{h}^{2h} \whiA_h I_{2h}^h\wb^{2h}_k =\left(\; 
(c_k^{2h})^2(1-\beta_h(\sigma_k))+(s_k^{2h})^2(1-\beta_h(\sigma_{k'}))\;\right)\wb_k^{2h}.\label{eq:projected_waveholtz_eig}
\end{equation}
with $k'=N-k$.
\end{thm}
\begin{proof}
Recall that eigenvectors of $L_h$ is also an eigenvector of $\whiA_h$ and satisfies \eqref{eq:waveholtz_eigvectors}. 
Utilizing equation \eqref{eq:full_weight} and \eqref{eq:waveholtz_eigvectors} we get
\begin{align}
\whiA_h I_{2h}^h\wb^{2h}_k &= \whiA_hc_k^{2h}\wb_k^h-\whiA_hs_k^{2h}\wb_{k'}^h\notag\\
&= (\;1-\beta(\sigma_k^h)\;)c_k^{2h}\wb_k^h-(\;1-\beta(\sigma_{k'}^h)\;)s_k^{2h}\wb_{k'}^h.
\end{align}
Then using \eqref{eq:prolong_k} and \eqref{eq:prolong_kp} we obtain
\begin{align}
I_{h}^{2h}\whiA_h I_{2h}^h\wb_{2h}^k &= (\;1-\beta(\sigma_k^h)\;)c_k^{2h}I_{h}^{2h}\wb_k^h-(\;1-\beta(\sigma_{k'}^h)\;)s_k^{2h}I_{h}^{2h}\wb_{k'}^h\notag\\
&=  (\;1-\beta(\sigma_k^h)\;)(c_k^{2h})^2\wb_k^{2h}+
(\;1-\beta(\sigma_{k'}^h)\;)(s_k^{2h})^2\wb_k^{2h}\notag\\
&=\left(\; 
(c_k^{2h})^2(1-\beta_h(\sigma_k))+(s_k^{2h})^2(1-\beta_h(\sigma_{k'}))\;\right)\wb_{k}^{2h}.
\end{align}
\end{proof}

Now we move to the multilevel case. The computation is similar but more involved.
\begin{thm}\label{thm:multilevel_eig}
Let $1\leq k<\frac{N}{2^{l}}$. Then the $k$-th eigenvector of the discrete Laplacian operator $L_{2^{l}h}$, $\wb_{k}^{2^lh}$, is an eigenvector of 
$I_{2^{l-1}h}^{2^lh}\dots I_{h}^{2h} \whiA_h I_{2h}^h\dots I_{2^lh}^{2^{l-1}h}$.
\end{thm}
\begin{proof}
Repeatedly using \eqref{eq:restri_prolong_equality}, we get
\begin{align*}
   I_{2^{l-1}h}^{2^lh}\dots I_{h}^{2h} \whiA_h I_{2h}^h\dots I_{2^lh}^{2^{l-1}h}w_{k}^{2^lh} &=
   I_{2^{l-1}h}^{2^lh}\dots I_{h}^{2h} \whiA_h I_{2h}^h\dots I_{2^{l-1}h}^{2^{l-2}h}
   \left(C_k^{(l)}\wb_{k}^{2^{l-1}h}+C_{\frac{N}{2^{l-1}}-k}^{(l)}\wb^{2^{l-1}h}_{\frac{N}{2^{l-1}}-k}\right)\notag\\
   &=I_{2^{l-1}h}^{2^lh}\dots I_{h}^{2h} \whiA_h
  \left( \sum_{j=1}^{2^{l-1}} C_{\frac{(j-1)N}{2^{l-1}}+k}^{(1)}\wb_{\frac{(j-1)N}{2^{l-1}}+k}^h
   +\sum_{j=1}^{2^{l-1}} C_{\frac{jN}{2^{l-1}}-k}^{(1)}\wb_{\frac{jN}{2^{l-1}}-k}^h\right)\notag\\
   &=I_{2^{l-1}h}^{2^lh}\dots I_{h}^{2h}\left( \sum_{j=1}^{2^{l-1}} \widetilde{C}_{\frac{(j-1)N}{2^{l-1}}+k}^{(1)}\wb_{\frac{(j-1)N}{2^{l-1}}+k}^h
   +\sum_{j=1}^{2^{l-1}} \widetilde{C}_{\frac{jN}{2^{l-1}}-k}^{(1)}\wb_{\frac{jN}{2^{l-1}}-k}^h\right)\notag\\
   &=I_{2^{l-1}h}^{2^lh}\dots I_{2h}^{4h}\left( \sum_{j=1}^{2^{l-2}} \hat{C}_{\frac{(j-1)N}{2^{l-1}}+k}^{(2)}\wb_{\frac{(j-1)N}{2^{l-1}}+k}^{2h}
   +\sum_{j=1}^{2^{l-2}} \hat{C}_{\frac{jN}{2^{l-1}}-k}^{(2)}\wb_{\frac{jN}{2^{l-1}}-k}^{2h}\right)\notag\\
   &= \hat{C}^{(l)}\wb_{k}^{2^lh},
\end{align*}
where all the $\hat{C}$, $\widetilde{C}$ and $C$ are generic constants. 
\end{proof}

A direct result of the variational property \eqref{eq:variational_property} and Theorem \ref{thm:multilevel_eig} is that eigenvectors of $W_{L-1}^T\dots W_1^T A_h W_1\dots W_{L-1}$ with $W_l=I_{2^{l+1}h}^{2^lh}$ are the eigenvectors of the discrete Laplacian operator $L_{2^{L}h}$. 

\subsubsection{Loss of Galerkin condition}
We also want to point out that the WaveHoltz operator $\whiA_h$ does not satisfy the Galerkin condition, in other words 
\begin{equation*}
    \whiA_{2h}\neq I_{h}^{2h}\whiA_hI_{2h}^h.
\end{equation*}
With the time stepping in \eqref{eq:modified_time_stepping} and the quadrature in \eqref{eq:quadrature} one can show that $\whiA_{h}\wb = P_{N_t}(L_h)\wb$ where 
$P_{N_t}(x)=\xi_0+\xi_1x+\dots+\xi_{N_t}x^{N_t}$ is a polynomial with $\xi_{N_t}\neq 0$.
If CFL conditions for the coarse grid $\Omega_{2h}$ and the fine grid $\Omega_h$ are the same, the total number of time steps will be different and $A_{2h}$ will be a polynomial of $L_{2h}$ but with adifferent degree. We can also use the same total number of time steps on the coarse level to get a modified coarse level WaveHoltz operator $\widetilde{\whiA}_{2h}=P_{N_t}(L_2h)$. Based on the Galerkin condition $L_{2h}=I_{h}^{2h}L_hI_{2h}^h$ we have
\begin{equation}
(L_{2h})^{n_t} = (I_{h}^{2h}L_hI_{2h}^h)^{n_t}= I_{h}^{2h}L_h (I_{2h}^hI_{h}^{2h})L_h\dots L_h(I_{2h}^hI_{h}^{2h})L_h I_{h}^{2h} \neq I_h^{2h} (L_h)^{n_t} I_{2h}^h,\quad \textrm{if} n_t\geq 1.
\end{equation}
 As a result $\widetilde{\whiA}_{2h}\neq I_{h}^{2h}\whiA_hI_{2h}^h$.
Without the Galerkin condition 
$\left(I_{h}^{2h}\whiA_h I_{2h}^h\right)^{-1}$ can not be inverted by directly applying the WaveHoltz solver on the coarse grid.

%%%%%%%%%%%%%%%%%%%%%%%%%%%%%%%%%%%%%
\begin{figure}
\begin{center}
\setlength{\unitlength}{0.8cm}
\begin{picture}(8,3) 
% Grid
\thicklines
\put(0,1){\line(1,0){8}}
\put(0,2){\line(1,0){8}}
% intervals on refined mesh
\put(0,2){\line(0,1){0.25}}
\put(1,2){\line(0,1){0.25}}
\put(2,2){\line(0,1){0.25}}
\put(3,2){\line(0,1){0.25}}
\put(4,2){\line(0,1){0.25}}
\put(5,2){\line(0,1){0.25}}
\put(6,2){\line(0,1){0.25}}
\put(7,2){\line(0,1){0.25}}
\put(8,2){\line(0,1){0.25}}
% intervalus on coarse mesh
\put(0,1){\line(0,1){0.25}}
\put(2,1){\line(0,1){0.25}}
\put(4,1){\line(0,1){0.25}}
\put(6,1){\line(0,1){0.25}}
\put(8,1){\line(0,1){0.25}}
% index for grid points on refined mesh
\put(-0.1,2.3){$0$}
\put(0.9,2.3){$1$} 
\put(1.9,2.3){$2$} 
\put(2.9,2.3){$3$} 
\put(3.9,2.3){$4$} 
\put(4.9,2.3){$5$} 
\put(5.9,2.3){$6$} 
\put(6.9,2.3){$7$} 
\put(7.9,2.3){$8$} 
% index for grid points on coarse mesh
\put(-0.1,1.3){$0$}
\put(1.9,1.3){$1$} 
\put(3.9,1.3){$2$} 
\put(5.9,1.3){$3$} 
\put(7.9,1.3){$4$} 
% text
\put(-1,2){$\Omega_h$:}
\put(-1,1){$\Omega_{2h}$:}
\end{picture}
\end{center}
\caption{The fine grid $\omega_h$ and the coarse grid $\omega_{2h}$ with $N=8$.\label{fig:fine-coarse-grid}}
\end{figure}
%%%%%%%%%%%%%%%%%%%%%%%%%%%%%%%%%%%%%

\section{Numerical verification}
To verify the theory in Sec. \ref{sec:iter_vs_eig}, we
consider two tests.

In the first test we consider the problem
\begin{align}
\omega^2 u +\Delta u = \omega^2\delta(\bx-\bx_c), \quad\bx\in[0,1]^d,\bx_c=(0.5,\dots,0.5)^T, d=2,3.
\end{align}
We consider $\omega=40,80$ in 2D with and $\omega=20,40$ in 3D, In each direction we use $N=2^{\lceil\log_2(\lceil 4\omega\rceil)\rceil}-1$ in 2D and $N=2^{\lceil\log_2(\lceil 2\omega\rceil)\rceil}-1$ grid points in 3D. In the deflation step we not only use eigenvectors from the original grid but also use the eigenvectors interpolated from one level and two level coarsen grids.

In Fig. \ref{fig:iter_vs_eig} we plot the number of iterations of the DCG method to reach the relative tolerance $10^{-7}$ as a function of the number of eigenvectors in the deflation space.
According to our theory if the number of eigenvalues $K$ scales as $O(\omega^s)$, the number of iterations for the convergence $N_{\textrm{iter}}$ scales as $O(\omega^{d-s})$. Under the $\log$-scale we have
\begin{equation}
    \log_{10}(K)\propto\log_{10}(\omega) s \quad\text{and}\quad
    \log_{10}(N_{\textrm{iter}})\propto \log_{10}(\omega)(d-s)=\log_{10}(\omega)d - \log_{10}(K),
\end{equation}
so $log_{10}(K)$-$\log_{10}(N_{\textrm{iter}})$ picture is a straight line with slope $-1$. 
In Fig. \ref{fig:iter_vs_deflation_dim} $N_{\textrm{iter}}$-$K$ can indeed be qualitatively captured by straight lines with slope $-1$ under the $\log$-scale with both exact eigenvectors and eigenvectors interpolated from one or two level coarsened grid. 

In the second test

\begin{figure}[htb]
\begin{center}
\includegraphics[width=0.46\textwidth,trim={0.0cm 0.0cm 0.0cm 0.0cm},clip]{figures/2d_eig_vs_iter_eig_orig_40.eps}
\includegraphics[width=0.46\textwidth,trim={0.0cm 0.0cm 0.0cm 0.0cm},clip]{figures/2d_eig_vs_iter_eig_orig_80.eps}
\includegraphics[width=0.46\textwidth,trim={0.0cm 0.0cm 0.0cm 0.0cm},clip]{figures/3d_eig_vs_iter_eig_orig_20.eps}
\includegraphics[width=0.46\textwidth,trim={0.0cm 0.0cm 0.0cm 0.0cm},clip]{figures/3d_eig_vs_iter_eig_orig_40.eps}
\caption{Number of iterations as a function of number of eigenvectors in the deflation space to reach relative error tolerance $10^{-7}$. \label{fig:iter_vs_eig}}
\end{center}
\end{figure}

\subsection{Complexity}
In this section we express the complexity with respect to estimated floating point operations and storage requirements. Throughout we assume that the discretization is done with a fixed number of points per wavelength. We give the complexity estimates both in terms of the frequency $\omega$ and the system size $N$. As will be seen some of the estimates are dimension dependent.   

\begin{table}[htbp]
  \centering
 \medskip
    \begin{tabular}{|l|c|c|c|c|c|c|c|c|c|c|c|}
    \hline
 	Apply $A$ & $W^TA r$ & $(W^TAW)^{-1}$ & $O(N)$ operations & Total cost & Memory \\ \hline
 	$N\times N_t$ & $k_\textrm{eig}\times N$ & $k_\textrm{eig}^2$ \textrm{or} $k_\textrm{eig}$ & $N$ & $k_\textrm{eig}\times N$ &
 	 $k_\textrm{eig}\times N$ \\ \hline
 	$\omega^d\times N_t$ & $\omega^{2d}$ & $\omega^{2d}$ or $\omega^d$ & $\omega^d$ &
 	$\omega^{2d}$ & $\omega^{2d}$\\ 
 	\hline
 	 $N\times N_t$ & $N^2$ & $N^{2}$ or $N$ & $N$ & $N^2$ & $N^2$\\
 	\hline
 \end{tabular}
      \caption{}
\end{table}

\begin{table}[htbp]
  \centering
 \medskip
    \begin{tabular}{|l|c|c|c|c|c|c|c|c|c|c|c|}
    \hline
 	Apply $A$ & $W^TA r$ & $(W^TAW)^{-1}$ & $O(N)$ operations & Total cost & Memory \\ \hline
 	$N\times N_t$ & $k_\textrm{eig}\times N$ & $k_\textrm{eig}^2$ \textrm{or} $k_\textrm{eig}$ & $N$ & $k_\textrm{eig}\times N$ &
 	 $k_\textrm{eig}\times N$ \\ \hline
 	$\omega^d\times N_t$ & $\omega^{d+s}$ & $\omega^{2s}$ or $\omega^{s}$ & $\omega^d$ &
 	$N_\textrm{iter}\omega^{d+s}$ & $\omega^{d+s}$\\ 
 	\hline
 	 $N\times N_t$ & $N^{1+s/d}$ & $N^{2s/d}$ or $N^{s/d}$ & $N$ & $N_\textrm{iter}\times N^{1+s/d}$ & $N^{1+s/d}$\\
 	\hline\hline
 	 	 $N\times N_t$ & $N$ & $1$  & $N$ & $N^2$ & $N$\\
 	\hline
 	 	 	 $N\times N_t$ & $N^{1+(d-1)/d}$ & $N^{2(d-1)/d}$ or $N^{(d-1)/d}$ & $N$ & $ N^2$ & $N^{1+(d-1)/d}$\\
 	 	 	 \hline
 \end{tabular}
      \caption{}
\end{table}

\begin{table}[htbp]
\scriptsize
\begin{center}
\begin{tabular}{|l|c|c|c|c|c|c|c|c|c|c|c|}
    \hline
 	& Apply $A$ & $W^TA r$ & $(W^TAW)^{-1}$ & Form $AW$ & Form $W$ & Total cost & Memory    \\ 
 	 	\hline
 	DCG & $NN_t$ & $N^{2}$ & $N^2$ or $N$ & $N_tN^2$ & $N_\textrm{arpack}$ & $N_\textrm{RHS}( N_\textrm{iter}N+ N^{2})+N_t N^2+N_\textrm{arpack}$ & $N^2$
 	 \\ \hline
 	DCG & $N N_t$ & $N^{1+s/d}$ & $N^{2s/d}$ or $N^{s/d}$ & $N_tN^{1+s/d}$ & $N_\textrm{arpack}$ & $N_\textrm{RHS}( N^{1-s/d}N+ N^{1+s/d}) +N_t N^{1+s/d}+N_\textrm{arpack}$& $N^{1+s/d}$
 	 \\ \hline
 	 DCG & $\omega^d N_t$ & $\omega^{d+s}$ & $\omega^{2s}$ or $\omega^s$ & $N_t\omega^{d+s}$ & $N_\textrm{arpack}$ & $N_\textrm{RHS}( \omega^{2d-s}+ \omega^{d+s}) +N_t \omega^{d+s}+N_\textrm{arpack}$& $\omega^{d+s}$
 	 \\ \hline
   CG & $N N_t$ & NA & NA & NA & NA & $N_\textrm{RHS}N^2$ & $N$ \\ \hline
   CG & $N N_t$ & NA & NA & NA & NA & $N_\textrm{RHS}\omega^{2d}$ & $N$ \\ \hline
 \end{tabular}
      \caption{}
 \end{center}
\end{table}
\normalsize

\begin{figure}[htb]
\begin{center}
\includegraphics[width=0.48\textwidth,trim={0.0cm 0.0cm 0.0cm 0.0cm},clip]{figures/neigs_vs_cputime_40_2d}
\includegraphics[width=0.48\textwidth,trim={0.0cm 0.0cm 0.0cm 0.0cm},clip]{figures/neigs_vs_cputime_30_3d}
\includegraphics[width=0.48\textwidth,trim={0.0cm 0.0cm 0.0cm 0.0cm},clip]{figures/neigs_vs_iter_40_2d}
\includegraphics[width=0.48\textwidth,trim={0.0cm 0.0cm 0.0cm 0.0cm},clip]{figures/neigs_vs_iter_30_3d}
\caption{CPU time and number of iterations for the KrylovKit (Krylov-Schur algorithm) to compute eigenvectors. Left: 2D. Right: 3D. \label{fig:eig_efficiency}}
\end{center}
\end{figure}

\subsection{Rate of convergence with and without deflation}

\begin{figure}[htb]
\begin{center}
\includegraphics[width=0.32\textwidth,trim={0.0cm 0.0cm 0.0cm 0.0cm},clip]{figures/2d_iter_vs_defdim}
\includegraphics[width=0.32\textwidth]{figures/3d_iter_vs_defdim}
\includegraphics[width=0.32\textwidth]{figures/3d_iter_vs_defdim_2}
\caption{Number of iterations for convergence for different dimensions of the deflation space. \label{fig:iter_vs_deflation_dim}}
\end{center}
\end{figure}

\subsection{Compression of matrices}
\subsubsection{Compression of $W$}
\subsubsection{Compression of $W^T \whiA$}

\clearpage

%%%%%%%%%%%%%%%%%%%%%%%%%%%%%%%%%%%%%%%%%%%%%%
\subsection{Experiments in One Dimension}
The eigenvalues and eigenvectors of the three point discretization $[-1, 2, -1]$ of the Laplacian on the unit square with a grid size $h=1/(n+1)$ with Dirichlet boundary conditions are
\begin{eqnarray}
    \lambda_k &= 2 \left(1-\cos \left(\frac{k \pi}{n+1}\right) \right),\ \ k = 1\ldots,n \\
    v_k[i] &= \sqrt{\frac{2}{n+1}} \sin\left(i\frac{k\pi}{n+1}\right),\ \  i = 1\ldots,n,\, k = 1\ldots,n. 
\end{eqnarray}

To test how well the deflation works with eigenvectors computed on a coarse grid and then interpolated to a fine grid we consider the grids with $n=2^l-1$ interior points. In this experiment we only consider the case when the course and the fine level are one level apart. 

In Fig. \ref{fig:conv_linear} and Fig. \ref{fig:conv_spline} we display the relative reduction in the Euclidean norm of each of the eigenvectors after one WaveHoltz iteration using $\omega = 30$. We also display the the square root of the WaveHoltz filter function 
\begin{equation}
\beta(\lambda;\omega) = \frac{\omega (3 \lambda^2+\omega^2) \sin \left(2 \pi \frac{\lambda}{\omega} \right)}{ (4 \pi (\lambda^3 - \lambda \omega^2)},
\end{equation}
and the relative reduction in the Euclidean norm of the error in the interpolated eigenvector with the part along the coarse eigenvector removed (deflated). To be precise, let $\mathcal{I}$ be the interpolation (prolongation) operator and $v^{\rm f}_k$ and $ v^{\rm c}_k$ be the $k$th eigenvectors on the fine and coarse grids. Then for each $\lambda_k$ on the coarse grid we display $ \| \Pi \delta_{\rm D} \| / \| \delta_{\rm D} \|$ where
\[
\delta_{\rm D} = v^{\rm f}_k -  \mathcal{I} v^{\rm c}_k. 
\]  

The two different figures display results using linear interpolation and spline interpolation.

As can be seen in both cases the WaveHoltz iteration is highly efficient in reducing the size of the error contribution orthogonal to the deflation subspace (in this case a single vector...).

It is also clear that the reduction is improved with increasing resolution but also on coarse meshes it is fairly good.

\begin{figure}[htb]
\begin{center}
\includegraphics[width=1.0\textwidth,trim={8.0cm 2.5cm 6.0cm 2.3cm},clip]{figures/conv_in_norm1D_linear}
\caption{Relative reduction in norm using deflation with interpolated eigenvectors. This figure is for linear interpolation. \label{fig:conv_linear}}
\end{center}
 \end{figure}

\begin{figure}[htb]
\begin{center}
\includegraphics[width=1.0\textwidth,trim={8.0cm 2.5cm 6.0cm 2.3cm},clip]{figures/conv_in_norm1D_spline}
\caption{Relative reduction in norm using deflation with interpolated eigenvectors. This figure is for spline interpolation. \label{fig:conv_spline}}
\end{center}
 \end{figure}
%%%%%%%%%%%%%%%%%%%%%%%%%%%%%%%%%

%%%%%%%%%%%%%%%%%%%%%%%%%%%%%%%%%

\clearpage
\subsection{Experiments in Two Dimensions}
\subsubsection{The unit square}
% This is computations using the file test2D_square.m
The eigenvalues and eigenvectors of the five point discretization of the Laplacian on the unit square with a grid size $h=1/(n+1)$ with Dirichlet boundary conditions are found by tensor products from the one dimensional case. 
%\begin{eqnarray}
%    \lambda_k &= 2 \left(1-\cos \left(\frac{k \pi}{n+1}\right) \right),\ \ k = 1\ldots,n \\
 %   v_k[i] &= \sqrt{\frac{2}{n+1}} \sin\left(i\frac{k\pi}{n+1}\right),\ \  i = 1\ldots,n,\, k = 1\ldots,n. 
%\end{eqnarray}

Let $n$ be odd, then we can prolongate these onto a grid with $n_{\rm f} = (n-1)/2+1$ points by injection and linear interpolation (i.e. averaging). 

In Fig. \ref{fig:unit_square1} we display the number of iterations needed to reach a relative tolerance of $10^{-12}$ for $\omega = 10,11,\ldots,70$ using $n = \lceil 4 \omega \rceil -1$ and with the number of eigenvalues in the deflation space being $\lceil 0.005N \rceil $. The figure to the right also includes the number of iterations needed for the standard CG algorithm.

We note that the computations only computed the eigenvectors by prolonging those from a coarser grid, the matrix $\matW^T \whiA$ was formed using the prolonged eigenvectors. We next consider the case when also $\matW^T \whiA$ is computed on a coarse grid.

\begin{figure}[htb]
\begin{center}
\includegraphics[width=0.45\textwidth,trim={0.0cm 0.0cm 0.0cm 0.0cm},clip]{figures/unit_square_iter2}
\includegraphics[width=0.45\textwidth,trim={0.0cm 0.0cm 0.0cm 0.0cm},clip]{figures/unit_square_iter1}
\caption{Number of iterations needed to reach tolerance $10^{-12}$ for deflation using eigenvalues/eigenvectors computed on the grid (DCG) and using prolongated eigenvectors computed on a grid coarsened by a factor of 2 (DCG-prolonged). To the right results for CG is included for reference.  \label{fig:unit_square1}}
\end{center}
 \end{figure}

\subsection{Experiments in Three Dimensions}
%%%%%%%%%%%%%%%%%%%%%%%%%%%%%%%
\clearpage

\subsection{Experiments on the $d$-dimensional unit cube}
In one dimension the eigenvalues and eigenvectors of the three-point center difference discretization $[-1,2,-1]$ of the Laplacian operator with a grid size $h=1/(n+1)$ with Dirichlet boundary conditions are
\begin{subequations}
    \begin{align}
        &\lambda_k = 2\left(1-\cos(\frac{k\pi}{n+1})\right),\;k=1,\dots,n,\\
        &\vb_k^n[i] =\sqrt{\frac{2}{n+1}}\sin\left(i\frac{k\pi}{n+1}\right),\;i=1,\dots,n,\;k=1,\dots,n. 
    \end{align}
\end{subequations}
Let the matrix corresponding to this discretization be $L^{\textrm{(1d)}}_n$. Then $5$-point and $7$-point central difference of the  Laplacian operator for the unit square in 2D and unit cube in 3D can be written as
\begin{equation}
L^{\textrm{(2d)}}_n=L^{\textrm{(1d)}}_n\otimes I_{n}+I_{n}\otimes L^{\textrm{(1d)}}_n \quad\text{and}\quad
L^{\textrm{(3d)}}_n=(L^{\textrm{(1d)}}_n\otimes I_{n})\otimes I_{n}+
(I_{n}\otimes L^{\textrm{(1d)}}_n )\otimes I_{n}+
I_{n}\otimes (I_{n}\otimes L^{\textrm{(1d)}}_n )
\end{equation}
respectively. 

To test the deflation with eigenvectors computed on a coarse mesh and then prolonged to a fine grid, we consider $n=2^l-1$ interior points along one direction.

Besides the original DCG algorithm, we also consider two modified version of it. We call the first modified version DCG-D. We invert the diagonal part of $W^TAW$, namely $\textrm{diag}(W^TAW)$, instead of $W^TAW$. With $A$ being SPD and $W$ being eigenvectors of $A$ $W^TAW$ is diagonal, however, when $W$ is constructed with prolonged eigenvectors $W^TAW$ is not exactly diagonal. In the second modified version of DCG we drop  $ {\bm \mu} \gets (\matW^T \whiA \matW)^{-1} (\matW^T \whiA \rb)$ in the inner loop of Algorithm \ref{alg:DCG}, and we call it DCG-OI.  

We investigate the relation between number of iterations for the relative residual below $10^{-7}$ and the dimension of deflation space. We consider a problem with point source on the center of the computational domain $[0,1]^d$ with $d=1,2,3$.  In 1D the number of grid points is $n=2^{\lceil\log_2(\lceil16\omega\rceil)\rceil}-1$. In 2D we use 
$n=2^{\lceil\log_2(\lceil4\omega\rceil)\rceil}-1$ grid points along one direction.

\textcolor{blue}{Comment on the observations.}
%%%%%%%%%%%%%%%%%%%%%%%%%%%%%%%%%%%%%%%%%%%%%%%%%%%%%%%%%%%%%%%%%%%%%%%%%%%%%%%%%%
\begin{figure}[htb]
\begin{center}
\includegraphics[width=0.32\textwidth,trim={0.0cm 0.0cm 0.0cm 0.0cm},clip]{figures/regular_geometry/1d_iter_eig1_orig.eps}
\includegraphics[width=0.32\textwidth,trim={0.0cm 0.0cm 0.0cm 0.0cm},clip]{figures/regular_geometry/1d_iter_eig1_diag.eps}
\includegraphics[width=0.32\textwidth,trim={0.0cm 0.0cm 0.0cm 0.0cm},clip]{figures/regular_geometry/1d_iter_eig1_no.eps}
%%%%%%%%%%%%%%%%%%%%%%%%%%%%%%%%%%%
\includegraphics[width=0.32\textwidth,trim={0.0cm 0.0cm 0.0cm 0.0cm},clip]{figures/regular_geometry/1d_iter_eig75_orig.eps}
\includegraphics[width=0.32\textwidth,trim={0.0cm 0.0cm 0.0cm 0.0cm},clip]{figures/regular_geometry/1d_iter_eig75_diag.eps}
\includegraphics[width=0.32\textwidth,trim={0.0cm 0.0cm 0.0cm 0.0cm},clip]{figures/regular_geometry/1d_iter_eig75_no.eps}
%%%%%%%%%%%%%%%%%%%%%%%%%%%%%%%%%%%
\includegraphics[width=0.32\textwidth,trim={0.0cm 0.0cm 0.0cm 0.0cm},clip]{figures/regular_geometry/1d_iter_eig5_orig.eps}
\includegraphics[width=0.32\textwidth,trim={0.0cm 0.0cm 0.0cm 0.0cm},clip]{figures/regular_geometry/1d_iter_eig5_diag.eps}
\includegraphics[width=0.32\textwidth,trim={0.0cm 0.0cm 0.0cm 0.0cm},clip]{figures/regular_geometry/1d_iter_eig5_no.eps}
%%%%%%%%%%%%%%%%%%%%%%%%%%%%%%%%%%%
\includegraphics[width=0.32\textwidth,trim={0.0cm 0.0cm 0.0cm 0.0cm},clip]{figures/regular_geometry/1d_iter_eig25_orig.eps}
\includegraphics[width=0.32\textwidth,trim={0.0cm 0.0cm 0.0cm 0.0cm},clip]{figures/regular_geometry/1d_iter_eig25_diag.eps}
\includegraphics[width=0.32\textwidth,trim={0.0cm 0.0cm 0.0cm 0.0cm},clip]{figures/regular_geometry/1d_iter_eig25_no.eps}
%%%%%%%%%%%%%%%%%%%%%%%%%%%%%%%%%%%
\caption{Number of iterations as a function of frequency on 1D unit interval.\label{fig:iter_vs_omega_1d}}
\end{center}
 \end{figure}
%%%%%%%%%%%%%%%%%%%%%%%%%%%%%%%%%%%%%%%%%%%%%%%%%%%%%%%%%%%%%%%%%%%%%%%%%%%%%%%%%%

%%%%%%%%%%%%%%%%%%%%%%%%%%%%%%%%%%%%%%%%%%%%%%%%%%%%%%%%%%%%%%%%%%%%%%%%%%%%%%%%%%
\begin{figure}[htb]
\begin{center}
\includegraphics[width=0.32\textwidth,trim={0.0cm 0.0cm 0.0cm 0.0cm},clip]{figures/regular_geometry/2d_iter_eig2_orig.eps}
\includegraphics[width=0.32\textwidth,trim={0.0cm 0.0cm 0.0cm 0.0cm},clip]{figures/regular_geometry/2d_iter_eig2_diag.eps}
\includegraphics[width=0.32\textwidth,trim={0.0cm 0.0cm 0.0cm 0.0cm},clip]{figures/regular_geometry/2d_iter_eig2_no.eps}
%%%%%%%%%%%%%%%%%%%%%%%%%%%%%%%%%%%
\includegraphics[width=0.32\textwidth,trim={0.0cm 0.0cm 0.0cm 0.0cm},clip]{figures/regular_geometry/2d_iter_eig15_orig.eps}
\includegraphics[width=0.32\textwidth,trim={0.0cm 0.0cm 0.0cm 0.0cm},clip]{figures/regular_geometry/2d_iter_eig15_diag.eps}
\includegraphics[width=0.32\textwidth,trim={0.0cm 0.0cm 0.0cm 0.0cm},clip]{figures/regular_geometry/2d_iter_eig15_no.eps}
%%%%%%%%%%%%%%%%%%%%%%%%%%%%%%%%%%%
\includegraphics[width=0.32\textwidth,trim={0.0cm 0.0cm 0.0cm 0.0cm},clip]{figures/regular_geometry/2d_iter_eig1_orig.eps}
\includegraphics[width=0.32\textwidth,trim={0.0cm 0.0cm 0.0cm 0.0cm},clip]{figures/regular_geometry/2d_iter_eig1_diag.eps}
\includegraphics[width=0.32\textwidth,trim={0.0cm 0.0cm 0.0cm 0.0cm},clip]{figures/regular_geometry/2d_iter_eig1_no.eps}
%%%%%%%%%%%%%%%%%%%%%%%%%%%%%%%%%%%
\includegraphics[width=0.32\textwidth,trim={0.0cm 0.0cm 0.0cm 0.0cm},clip]{figures/regular_geometry/2d_iter_eig05_orig.eps}
\includegraphics[width=0.32\textwidth,trim={0.0cm 0.0cm 0.0cm 0.0cm},clip]{figures/regular_geometry/2d_iter_eig05_diag.eps}
\includegraphics[width=0.32\textwidth,trim={0.0cm 0.0cm 0.0cm 0.0cm},clip]{figures/regular_geometry/2d_iter_eig05_no.eps}
%%%%%%%%%%%%%%%%%%%%%%%%%%%%%%%%%%%
\caption{Number of iterations as a function of frequency on 2D unit square.\label{fig:iter_vs_omega_1d}}
\end{center}
 \end{figure}
%%%%%%%%%%%%%%%%%%%%%%%%%%%%%%%%%%%%%%%%%%%%%%%%%%%%%%%%%%%%%%%%%%%%%%%%%%%%%%%%%%

\newpage

Line 17: 
\begin{align}
W^TAW=D+B=D+U\Sigma U^T
=UDU^T+U\Sigma U^T
= U(D+\Sigma)U^T\\
 U(D+\Sigma)^{-1}U^T\\
D^{-1}W^TAW=D^{-1}(D+U\Sigma U^T)
= I + D^{-1} U\Sigma U^T
\end{align}
Von-Neumann series converges fast.
%\end{comment}
